# Supplementary material for: Good-for-Game QPTL: An Alternating Hodges Semantics
Source: arXiv:2104.06085 source file (2021-06-24)
Supplement: Supplementary file 1 [file AppendixE.tex]

%%****************************************************************************%%
%%                                                                            %%
%% Article Title                                                              %%
%%                                                                            %%
%% AppendixE.tex                                                              %%
%%                                                                            %%
%% Revision 0                                                                 %%
%%                                                                            %%
%% Copyright (C) 20xx, Fabio Mogavero.                                        %%
%% All rights reserved.                                                       %%
%%                                                                            %%
%%****************************************************************************%%

% Begin of file AppendixE.tex

\subsection{Proofs for Section~\ref{sec:expsuc}}
\label{app:expsuc}

\cbstart
...
\cbend

% End of file AppendixE.tex

%%% Local Variables:
%%% mode: latex
%%% TeX-master: "Article"
%%% End:
